# Supplementary material for: Extent of Fock-exchange mixing for a hybrid van der Waals density functional?
Source: arXiv:1805.04936 source file (2018-05-13)
Supplement: Supplementary file 1 [file SI.pdf]

# Supplementary materials – Extent of Fock-exchange mixing for a hybrid van der Waals density functional?

Yang Jiao,<sup>1</sup> Elsebeth Schröder,<sup>1</sup> and Per Hyldgaard<sup>1,\*</sup>

<sup>1</sup>*Department of Microtechnology and Nanoscience, MC2,  
Chalmers University of Technology, SE-41296 Gteborg, Sweden*

---

\* [hyldgaar@chalmers.se](mailto:hyldgaar@chalmers.se)

<sup>1</sup> L. A. Curtiss, K. Raghavachari, P. C. Redfern, and J. A. Pople, The Journal of Chemical Physics **106**, 1063 (1997), <http://dx.doi.org/10.1063/1.473182>.

<sup>2</sup> L. Goerigk, A. Hansen, C. Bauer, S. Ehrlich, A. Najibi, and S. Grimme, Phys. Chem. Chem. Phys. **19**, 32184 (2017).

<sup>3</sup> L. Goerigk and S. Grimme, J. Chem. Theory Comput. **6**, 107 (2010), pMID: 26614324.

<sup>4</sup> P. Jurecka, J. Sponer, J. Cerny, and P. Hobza, Phys. Chem. Chem. Phys. **8**, 1985 (2006).

<sup>5</sup> M. S. Marshall, L. A. Burns, and C. D. Sherrill, J. Chem. Phys. **135**, 194102 (2011), <https://doi.org/10.1063/1.3659142>.

TABLE S.I. Atomization energies (39 molecules from the G2-1 data set<sup>1</sup>). All energies in kcal/mol. This calculation uses vdW-DF-cx orbitals for  $\Delta E^{\text{tlh}}$ , which is only meaningful for this subset of the G2-1 benchmark set. Atomization energies at listed reference geometries (at relaxed geometries) are listed outside (inside) brackets. The first subgroup corresponds to cases with a downward concave coupling-constant variation, where  $\Delta E^{\text{tlh}}$  is calculated using Eq. (19). The second subgroup corresponds to cases with an upward concave coupling-constant variation, where  $\Delta E^{\text{tlh}}$  is calculated using Eq. (20). The two-legged constructions and the  $\Delta E^{\text{tlh}}$  results are not necessarily accurate for the second subgroup where the Fock-exchange mixing coefficient  $a_{\text{sys}}$  is large. Accordingly we provide estimates for the average  $a_{\text{sys}}$  values, for the mean absolute deviation (MAD) and for the mean absolute relative deviation (MARD) separately. We do, however, also include an overall, such characterization at the bottom of the table.

|                                | $\Delta E^{\text{Fo}}_{\text{x}}$ | $\Delta E^{\text{cx}}_{\text{x}}$ | $\Delta E^{\text{cx}}_{\text{xc}}$ | $\Delta E^{\text{cx}}_{\text{xc}, \lambda=1}$ | $\Delta E^{\text{cx}}$ | $\Delta E^{\text{tlh}}$ | $\Delta E^{\text{cx0}}$ | $\Delta E^{\text{ref}}$ | $a_{\text{sys}}$ |
|--------------------------------|-----------------------------------|-----------------------------------|------------------------------------|-----------------------------------------------|------------------------|-------------------------|-------------------------|-------------------------|------------------|
| LiH                            | 27                                | 28                                | 51                                 | 64                                            | 58[ 58]                | 57                      | 57[ 57]                 | 58                      | 0.23             |
| NH                             | 17                                | 27                                | 54                                 | 72                                            | 87[ 87]                | 85                      | 84[ 84]                 | 84                      | 0.22             |
| NH <sub>2</sub>                | 49                                | 69                                | 121                                | 155                                           | 187[ 187]              | 183                     | 182[ 182]               | 182                     | 0.22             |
| NH <sub>3</sub>                | 99                                | 127                               | 202                                | 252                                           | 303[ 303]              | 297                     | 296[ 296]               | 298                     | 0.22             |
| OH                             | -81                               | 28                                | 55                                 | 73                                            | 105[ 105]              | 92                      | 106[ 105]               | 106                     | 0.12             |
| H <sub>2</sub> O               | 80                                | 110                               | 160                                | 193                                           | 237[ 237]              | 230                     | 229[ 229]               | 233                     | 0.21             |
| HF                             | 52                                | 74                                | 98                                 | 115                                           | 145[ 150]              | 141                     | 139[ 140]               | 141                     | 0.20             |
| PH <sub>2</sub>                | 37                                | 43                                | 90                                 | 119                                           | 160[ 160]              | 158                     | 158[ 158]               | 153                     | 0.23             |
| PH <sub>3</sub>                | 65                                | 73                                | 141                                | 184                                           | 247[ 247]              | 245                     | 245[ 245]               | 242                     | 0.23             |
| Li <sub>2</sub>                | -5                                | -3                                | 11                                 | 18                                            | 19[ 19]                | 19                      | 19[ 19]                 | 24                      | 0.21             |
| LiF                            | 98                                | 124                               | 148                                | 165                                           | 140[ 145]              | 135                     | 134[ 134]               | 138                     | 0.19             |
| N <sub>2</sub>                 | -65                               | 6                                 | 59                                 | 97                                            | 228[ 230]              | 215                     | 211[ 214]               | 228                     | 0.18             |
| N <sub>2</sub> H <sub>4</sub>  | 143                               | 203                               | 331                                | 417                                           | 449[ 450]              | 436                     | 435[ 435]               | 438                     | 0.22             |
| NO                             | -118                              | 30                                | 73                                 | 105                                           | 161[ 161]              | 141                     | 144[ 145]               | 153                     | 0.13             |
| O <sub>2</sub>                 | -54                               | 32                                | 61                                 | 83                                            | 138[ 138]              | 125                     | 116[ 119]               | 120                     | 0.14             |
| H <sub>2</sub> O <sub>2</sub>  | 43                                | 123                               | 195                                | 244                                           | 281[ 281]              | 266                     | 261[ 262]               | 269                     | 0.19             |
| F <sub>2</sub>                 | -65                               | 10                                | 27                                 | 41                                            | 52[ 61]                | 43                      | 34[ 34]                 | 38                      | 0.12             |
| CO <sub>2</sub>                | 206                               | 213                               | 277                                | 325                                           | 408[ 408]              | 406                     | 378[ 380]               | 389                     | 0.24             |
| Na <sub>2</sub>                | -12                               | -7                                | 5                                  | 11                                            | 15[ 15]                | 14                      | 14[ 14]                 | 17                      | 0.20             |
| P <sub>2</sub>                 | -60                               | -13                               | 30                                 | 60                                            | 120[ 121]              | 112                     | 109[ 110]               | 117                     | 0.19             |
| ClO                            | -6                                | 36                                | 60                                 | 78                                            | 78[ 79]                | 71                      | 62[ 64]                 | 65                      | 0.17             |
| SO <sub>2</sub>                | 104                               | 153                               | 212                                | 256                                           | 277[ 279]              | 267                     | 243[ 247]               | 258                     | 0.20             |
| Average $a_{\text{sys}}$       |                                   |                                   |                                    |                                               |                        |                         |                         |                         | 0.19             |
| MAD(kcal/mol)                  |                                   |                                   |                                    |                                               | 7.35[ 8.40]            | 5.37                    | 5.14[ 4.36]             |                         |                  |
| MARD(%)                        |                                   |                                   |                                    |                                               | 6.92[ 8.42]            | 5.33                    | 4.74[ 4.22]             |                         |                  |
| BeH                            | 69                                | 67                                | 78                                 | 85                                            | 61[ 61]                | 62                      | 62[ 62]                 | 50                      | 0.18             |
| CH <sub>3</sub>                | 272                               | 180                               | 242                                | 282                                           | 317[ 317]              | 348                     | 311[ 311]               | 307                     | 0.34             |
| CH <sub>4</sub>                | 310                               | 222                               | 307                                | 362                                           | 429[ 429]              | 451                     | 423[ 423]               | 420                     | 0.25             |
| SiH <sub>2-S1A1d</sub>         | 122                               | 63                                | 104                                | 130                                           | 155[ 155]              | 174                     | 129[ 154]               | 151                     | 0.32             |
| SiH <sub>3</sub>               | 176                               | 110                               | 165                                | 199                                           | 232[ 232]              | 250                     | 232[ 232]               | 225                     | 0.27             |
| SiH <sub>4</sub>               | 211                               | 141                               | 218                                | 265                                           | 326[ 326]              | 342                     | 327[ 327]               | 322                     | 0.23             |
| SH <sub>2</sub>                | 140                               | 75                                | 117                                | 145                                           | 190[ 190]              | 213                     | 183[ 183]               | 182                     | 0.36             |
| C <sub>2</sub> H <sub>4</sub>  | 490                               | 326                               | 436                                | 510                                           | 579[ 579]              | 636                     | 563[ 564]               | 563                     | 0.34             |
| C <sub>2</sub> H <sub>6</sub>  | 583                               | 410                               | 556                                | 653                                           | 730[ 730]              | 778                     | 717[ 717]               | 712                     | 0.28             |
| CN                             | 126                               | 94                                | 136                                | 167                                           | 188[ 189]              | 195                     | 168[ 168]               | 181                     | 0.24             |
| HCN                            | 163                               | 125                               | 188                                | 232                                           | 320[ 321]              | 328                     | 301[ 303]               | 313                     | 0.21             |
| CO                             | 144                               | 101                               | 137                                | 164                                           | 265[ 266]              | 278                     | 248[ 249]               | 259                     | 0.30             |
| HCO                            | 188                               | 150                               | 202                                | 239                                           | 294[ 294]              | 302                     | 275[ 276]               | 279                     | 0.23             |
| H <sub>2</sub> CO              | 245                               | 203                               | 277                                | 327                                           | 387[ 387]              | 395                     | 369[ 370]               | 374                     | 0.21             |
| CH <sub>3</sub> OH             | 346                               | 292                               | 402                                | 476                                           | 526[ 526]              | 537                     | 512[ 512]               | 513                     | 0.20             |
| SiO                            | 88                                | 82                                | 115                                | 139                                           | 195[ 195]              | 196                     | 179[ 181]               | 192                     | 0.19             |
| SO                             | 87                                | 73                                | 99                                 | 119                                           | 141[ 142]              | 144                     | 122[ 124]               | 125                     | 0.22             |
| Si <sub>2</sub> H <sub>6</sub> | 382                               | 249                               | 378                                | 459                                           | 539[ 539]              | 571                     | 538[ 539]               | 530                     | 0.24             |
| CH <sub>3</sub> SH             | 412                               | 263                               | 367                                | 436                                           | 490[ 490]              | 540                     | 476[ 476]               | 474                     | 0.33             |
| HOCl                           | 131                               | 96                                | 139                                | 170                                           | 177[ 177]              | 185                     | 161[ 162]               | 164                     | 0.23             |
| Average $a_{\text{sys}}$       |                                   |                                   |                                    |                                               |                        |                         |                         |                         | 0.26             |
| MAD(kcal/mol)                  |                                   |                                   |                                    |                                               | 10.13[ 10.36]          | 29.38                   | 6.73[ 5.31]             |                         |                  |
| MARD(%)                        |                                   |                                   |                                    |                                               | 4.51[ 4.62]            | 10.26                   | 3.90[ 3.02]             |                         |                  |
| Average $a_{\text{sys}}$       |                                   |                                   |                                    |                                               |                        |                         |                         |                         | 0.22             |
| MAD(kcal/mol)                  |                                   |                                   |                                    |                                               | 8.67[ 9.34]            | 16.81                   | 5.90[ 4.81]             |                         |                  |
| MARD(%)                        |                                   |                                   |                                    |                                               | 5.77[ 6.61]            | 7.68                    | 4.34[ 3.65]             |                         |                  |

TABLE S.II. Atomization energies  $\Delta E$  for molecules in the G2-1 data set,<sup>1</sup> at listed reference geometries, using Hartree-Fock orbitals in  $\Delta E^{\text{tlh}}$ . Results at relaxed geometries are listed in brackets. The subgroups are organized as in Table S.I.

|                                                   | $\Delta E_x^{\text{HF}}$ | $\Delta E_x^{\text{cx}}$ | $\Delta E_{\text{xc}}^{\text{cx}}$ | $\Delta E_{\text{xc},\lambda=1}^{\text{cx}}$ | $\Delta E^{\text{cx}}$ | $\Delta E^{\text{tlh}}$ | $\Delta E^{\text{cx0}}$ | $\Delta E^{\text{ref}}$ | $a_{\text{sys}}$ |
|---------------------------------------------------|--------------------------|--------------------------|------------------------------------|----------------------------------------------|------------------------|-------------------------|-------------------------|-------------------------|------------------|
| BeH                                               | 7                        | 67                       | 78                                 | 85                                           | 61[ 61]                | 55                      | 62[ 62]                 | 50                      | 0.10             |
| CH                                                | 88                       | 114                      | 119                                | 124                                          | 77[ 77]                | 74                      | 71[ 72]                 | 84                      | 0.11             |
| CH <sub>2</sub> -s <sub>3</sub> B <sub>1</sub> d  | 111                      | 146                      | 182                                | 205                                          | 201[ 201]              | 194                     | 196[ 196]               | 190                     | 0.19             |
| CH <sub>2</sub> -s <sub>1</sub> A <sub>1</sub> d  | 101                      | 138                      | 172                                | 195                                          | 191[ 201]              | 184                     | 185[ 196]               | 181                     | 0.19             |
| CH <sub>3</sub>                                   | 135                      | 180                      | 242                                | 282                                          | 317[ 317]              | 308                     | 311[ 311]               | 307                     | 0.20             |
| CH <sub>4</sub>                                   | 168                      | 222                      | 307                                | 362                                          | 429[ 429]              | 418                     | 423[ 423]               | 420                     | 0.21             |
| NH                                                | 15                       | 27                       | 54                                 | 72                                           | 87[ 87]                | 84                      | 84[ 84]                 | 84                      | 0.22             |
| NH <sub>2</sub>                                   | 40                       | 69                       | 121                                | 155                                          | 187[ 187]              | 181                     | 182[ 182]               | 182                     | 0.21             |
| NH <sub>3</sub>                                   | 82                       | 127                      | 202                                | 252                                          | 303[ 303]              | 293                     | 296[ 296]               | 298                     | 0.21             |
| H <sub>2</sub> O                                  | 67                       | 110                      | 160                                | 193                                          | 237[ 237]              | 228                     | 229[ 229]               | 233                     | 0.20             |
| HF                                                | 39                       | 74                       | 98                                 | 115                                          | 145[ 150]              | 139                     | 139[ 140]               | 141                     | 0.18             |
| SiH <sub>2</sub> -s <sub>1</sub> A <sub>1</sub> d | 62                       | 63                       | 104                                | 130                                          | 155[ 155]              | 155                     | 129[ 154]               | 151                     | 0.23             |
| SiH <sub>2</sub> -s <sub>3</sub> B <sub>1</sub> d | 71                       | 84                       | 115                                | 135                                          | 138[ 138]              | 136                     | 137[ 138]               | 131                     | 0.22             |
| SiH <sub>3</sub>                                  | 99                       | 110                      | 165                                | 199                                          | 232[ 232]              | 230                     | 232[ 232]               | 225                     | 0.23             |
| SiH <sub>4</sub>                                  | 131                      | 141                      | 218                                | 265                                          | 326[ 326]              | 324                     | 327[ 327]               | 322                     | 0.23             |
| PH <sub>2</sub>                                   | 38                       | 43                       | 90                                 | 119                                          | 160[ 160]              | 159                     | 158[ 158]               | 153                     | 0.23             |
| PH <sub>3</sub>                                   | 63                       | 73                       | 141                                | 184                                          | 247[ 247]              | 245                     | 245[ 245]               | 242                     | 0.23             |
| SH <sub>2</sub>                                   | 28                       | 75                       | 117                                | 145                                          | 190[ 190]              | 181                     | 183[ 183]               | 182                     | 0.19             |
| HCl                                               | 13                       | 52                       | 73                                 | 86                                           | 110[ 111]              | 104                     | 106[ 106]               | 106                     | 0.16             |
| LiF                                               | 111                      | 124                      | 148                                | 165                                          | 140[ 145]              | 137                     | 134[ 134]               | 138                     | 0.21             |
| C <sub>2</sub> H <sub>2</sub>                     | 112                      | 237                      | 310                                | 361                                          | 417[ 417]              | 395                     | 398[ 399]               | 406                     | 0.17             |
| C <sub>2</sub> H <sub>4</sub>                     | 212                      | 326                      | 436                                | 510                                          | 579[ 579]              | 557                     | 563[ 564]               | 563                     | 0.19             |
| C <sub>2</sub> H <sub>6</sub>                     | 307                      | 410                      | 556                                | 653                                          | 730[ 730]              | 709                     | 717[ 717]               | 712                     | 0.21             |
| CN                                                | 51                       | 94                       | 136                                | 167                                          | 188[ 189]              | 179                     | 168[ 168]               | 181                     | 0.19             |
| HCN                                               | 11                       | 125                      | 188                                | 232                                          | 320[ 321]              | 301                     | 301[ 303]               | 313                     | 0.17             |
| CO                                                | 5                        | 101                      | 137                                | 164                                          | 265[ 266]              | 251                     | 248[ 249]               | 259                     | 0.15             |
| HCO                                               | 57                       | 150                      | 202                                | 239                                          | 294[ 294]              | 278                     | 275[ 276]               | 279                     | 0.17             |
| H <sub>2</sub> CO                                 | 104                      | 203                      | 277                                | 327                                          | 387[ 387]              | 369                     | 369[ 370]               | 374                     | 0.18             |
| CH <sub>3</sub> OH                                | 201                      | 292                      | 402                                | 476                                          | 526[ 526]              | 508                     | 512[ 512]               | 513                     | 0.20             |
| N <sub>2</sub>                                    | -96                      | 6                        | 59                                 | 97                                           | 228[ 230]              | 211                     | 211[ 214]               | 228                     | 0.17             |
| N <sub>2</sub> H <sub>4</sub>                     | 117                      | 203                      | 331                                | 417                                          | 449[ 450]              | 432                     | 435[ 435]               | 438                     | 0.21             |
| NO                                                | -41                      | 30                       | 73                                 | 105                                          | 161[ 161]              | 148                     | 144[ 145]               | 153                     | 0.17             |
| O <sub>2</sub>                                    | -24                      | 32                       | 61                                 | 83                                           | 138[ 138]              | 128                     | 116[ 119]               | 120                     | 0.17             |
| H <sub>2</sub> O <sub>2</sub>                     | 21                       | 123                      | 195                                | 244                                          | 281[ 281]              | 263                     | 261[ 262]               | 269                     | 0.18             |
| F <sub>2</sub>                                    | -95                      | 10                       | 27                                 | 41                                           | 52[ 61]                | 42                      | 34[ 34]                 | 38                      | 0.10             |
| CO <sub>2</sub>                                   | 65                       | 213                      | 277                                | 325                                          | 408[ 408]              | 385                     | 378[ 380]               | 389                     | 0.16             |
| Si <sub>2</sub>                                   | -14                      | 47                       | 67                                 | 81                                           | 82[ 82]                | 74                      | 74[ 75]                 | 75                      | 0.14             |
| P <sub>2</sub>                                    | -68                      | -13                      | 30                                 | 60                                           | 120[ 121]              | 110                     | 109[ 110]               | 117                     | 0.18             |
| S <sub>2</sub>                                    | -26                      | 68                       | 91                                 | 108                                          | 121[ 121]              | 109                     | 104[ 104]               | 102                     | 0.12             |
| Cl <sub>2</sub>                                   | -18                      | 60                       | 77                                 | 89                                           | 70[ 70]                | 61                      | 57[ 58]                 | 58                      | 0.11             |
| NaCl                                              | 74                       | 84                       | 103                                | 115                                          | 96[ 96]                | 93                      | 92[ 93]                 | 98                      | 0.21             |
| SiO                                               | 13                       | 82                       | 115                                | 139                                          | 195[ 195]              | 183                     | 179[ 181]               | 192                     | 0.16             |
| CS                                                | -37                      | 75                       | 105                                | 127                                          | 181[ 181]              | 166                     | 162[ 162]               | 171                     | 0.13             |
| SO                                                | -17                      | 73                       | 99                                 | 119                                          | 141[ 142]              | 129                     | 122[ 124]               | 125                     | 0.13             |
| ClO                                               | -6                       | 36                       | 60                                 | 78                                           | 78[ 79]                | 71                      | 62[ 64]                 | 65                      | 0.17             |
| ClF                                               | -22                      | 57                       | 74                                 | 88                                           | 74[ 79]                | 65                      | 59[ 61]                 | 61                      | 0.12             |
| Si <sub>2</sub> H <sub>6</sub>                    | 227                      | 249                      | 378                                | 459                                          | 539[ 539]              | 534                     | 538[ 539]               | 530                     | 0.23             |
| CH <sub>3</sub> Cl                                | 151                      | 237                      | 319                                | 374                                          | 408[ 408]              | 392                     | 396[ 397]               | 394                     | 0.19             |
| CH <sub>3</sub> SH                                | 168                      | 263                      | 367                                | 436                                          | 490[ 490]              | 471                     | 476[ 476]               | 474                     | 0.20             |
| HOCl                                              | 7                        | 96                       | 139                                | 170                                          | 177[ 177]              | 162                     | 161[ 162]               | 164                     | 0.16             |
| SO <sub>2</sub>                                   | -4                       | 153                      | 212                                | 256                                          | 277[ 279]              | 254                     | 243[ 247]               | 258                     | 0.15             |
| Average $a_{\text{sys}}$                          |                          |                          |                                    |                                              |                        |                         |                         |                         | 0.18             |
| MAD(kcal/mol)                                     |                          |                          |                                    |                                              | 9.48[ 10.33]           | 4.56                    | 5.83[ 5.08]             |                         |                  |
| MARD(%)                                           |                          |                          |                                    |                                              | 6.36[ 7.32]            | 2.96                    | 3.70[ 3.16]             |                         |                  |
| LiH                                               | 31                       | 28                       | 51                                 | 64                                           | 58[ 58]                | 58                      | 57[ 57]                 | 58                      | 0.13             |
| OH                                                | 31                       | 28                       | 55                                 | 73                                           | 105[ 105]              | 106                     | 106[ 105]               | 106                     | 0.17             |
| Li <sub>2</sub>                                   | 16                       | -3                       | 11                                 | 18                                           | 19[ 19]                | 24                      | 19[ 19]                 | 24                      | 0.27             |
| Na <sub>2</sub>                                   | 8                        | -7                       | 5                                  | 11                                           | 15[ 15]                | 19                      | 14[ 14]                 | 17                      | 0.24             |
| Average $a_{\text{sys}}$                          |                          |                          |                                    |                                              |                        |                         |                         |                         | 0.20             |
| MAD(kcal/mol)                                     |                          |                          |                                    |                                              | 2.06[ 2.02]            | 0.74                    | 2.38[ 2.55]             |                         |                  |
| MARD(%)                                           |                          |                          |                                    |                                              | 7.94[ 7.84]            | 3.27                    | 10.15[ 10.28]           |                         |                  |
| Average $a_{\text{sys}}$                          |                          |                          |                                    |                                              |                        |                         |                         |                         | 0.18             |
| MAD(kcal/mol)                                     |                          |                          |                                    |                                              | 8.94[ 9.73]            | 4.29                    | 5.58[ 4.90]             |                         |                  |
| MARD(%)                                           |                          |                          |                                    |                                              | 6.47[ 7.36]            | 2.98                    | 4.17[ 3.68]             |                         |                  |

TABLE S.III. Reaction energies (17 reactions from the G2RC data set<sup>2</sup>) at listed reference geometries. All energies in kcal/mol. This calculation uses vdW-DF-cx orbitals for  $\Delta E^{\text{tlh}}$ , which is only meaningful for this subset of the G2RC benchmark set. Reaction energies at relaxed geometries are listed in brackets, where available. Organization of data split into two subgroups depending on the nature of the vdW-DF-tlh construction, as in Table S.I.

|                                                                                               | $\Delta E_x^{\text{Fo}}$ | $\Delta E_x^{\text{cx}}$ | $\Delta E_{\text{xc}}^{\text{cx}}$ | $\Delta E_{\text{xc}, \lambda=1}^{\text{cx}}$ | $\Delta E^{\text{cx}}$ | $\Delta E^{\text{tlh}}$ | $\Delta E^{\text{cx0}}$ | $\Delta E^{\text{ref}}$ | $a_{\text{sys}}$ |
|-----------------------------------------------------------------------------------------------|--------------------------|--------------------------|------------------------------------|-----------------------------------------------|------------------------|-------------------------|-------------------------|-------------------------|------------------|
| $\text{C}_2\text{H}_6\text{OS} \rightarrow \text{C}_2\text{H}_4\text{S} + \text{H}_2\text{O}$ | 13                       | 23                       | 32                                 | 39                                            | 1.97[ 2.04]            | 0.06                    | 0.07[ 0.71]             | -2.23                   | 0.19             |
| $\text{C}_2\text{H}_4\text{O} \rightarrow \text{CO} + \text{CH}_4$                            | 55                       | 63                       | 77                                 | 87                                            | 4.98[ 5.03]            | 3.24                    | 3.22[ 3.23]             | -2.18                   | 0.21             |
| $\text{H}_6\text{Si}_2 + \text{H}_2 \rightarrow 2\text{H}_4\text{Si}$                         | -13                      | -6                       | -3                                 | -1                                            | -1.54[ -1.50]          | -2.63                   | -3.32[ -3.27]           | -4.10                   | 0.15             |
| $\text{CO} + \text{H}_2\text{O} \rightarrow \text{CO}_2 + \text{H}_2$                         | -13                      | -33                      | -38                                | -42                                           | -18.11[ -18.13]        | -15.67                  | -13.46[ -13.51]         | -7.10                   | 0.12             |
| $\text{C}_2\text{H}_3\text{N} + \text{H}_2\text{O} \rightarrow \text{C}_2\text{H}_5\text{NO}$ | -61                      | -62                      | -78                                | -90                                           | -27.18[ -27.16]        | -26.87                  | -27.22[ -27.24]         | -19.47                  | 0.24             |
| $\text{BCl}_3 + \text{AlF}_3 \rightarrow \text{BF}_3 + \text{AlCl}_3$                         | -17                      | -2                       | -1                                 | -2                                            | -25.51[ -25.53]        | -26.61                  | -29.30[ -29.61]         | -27.15                  | 0.07             |
| $\text{N}_2\text{O} + \text{H}_2 \rightarrow \text{N}_2 + \text{H}_2\text{O}$                 | -54                      | -9                       | -5                                 | -3                                            | -62.25[ -62.16]        | -64.88                  | -73.11[ -73.04]         | -81.21                  | 0.06             |
| $\text{C}_2\text{H}_4 + \text{CH}_2 \rightarrow \text{C}_3\text{H}_6$                         | -73                      | -78                      | -112                               | -136                                          | -111.08[ -100.41]      | -109.86                 | -109.80[ -98.65]        | -109.11                 | 0.23             |
| Average $a_{\text{sys}}$                                                                      |                          |                          |                                    |                                               |                        |                         |                         |                         | 0.16             |
| MAD(kcal/mol)                                                                                 |                          |                          |                                    |                                               | 6.90[ 7.77]            | 5.35                    | 4.19[ 5.56]             |                         |                  |
| MARD(%)                                                                                       |                          |                          |                                    |                                               | 100.67[ 102.22]        | 71.10                   | 64.71[ 69.90]           |                         |                  |
| $\text{CO}_2 + \text{H}_2 \rightarrow \text{CH}_2\text{O}_2$                                  | -43                      | -35                      | -44                                | -51                                           | -0.12[ -0.13]          | -2.50                   | -2.32[ -2.29]           | -2.26                   | 0.27             |
| $\text{C}_2\text{H}_2 + \text{HF} \rightarrow \text{C}_2\text{H}_3\text{F}$                   | -39                      | -39                      | -51                                | -60                                           | -32.98[ -33.00]        | -32.98                  | -33.36[ -33.37]         | -26.97                  | 0.18             |
| $\text{CH}_2\text{O} + \text{H}_2 \rightarrow \text{CH}_4\text{O}$                            | -65                      | -54                      | -64                                | -71                                           | -27.25[ -27.25]        | -30.53                  | -29.89[ -29.92]         | -29.46                  | 0.30             |
| $\text{C}_2\text{H}_2 + \text{C}_2\text{H}_4 \rightarrow \text{C}_4\text{H}_6$                | -75                      | -72                      | -94                                | -111                                          | -39.67[ -39.71]        | -40.31                  | -40.68[ -40.79]         | -32.71                  | 0.19             |
| $\text{N}_2 + 3\text{H}_2 \rightarrow 2\text{H}_3\text{N}$                                    | -149                     | -137                     | -155                               | -169                                          | -38.79[ -38.79]        | -41.67                  | -41.60[ -41.55]         | -39.43                  | 0.25             |
| $\text{C}_2\text{H}_2 + \text{H}_2 \rightarrow \text{C}_2\text{H}_4$                          | -63                      | -54                      | -64                                | -71                                           | -50.15[ -50.16]        | -52.58                  | -52.44[ -52.41]         | -49.20                  | 0.27             |
| $\text{CO} + 3\text{H}_2 \rightarrow \text{H}_2\text{O} + \text{CH}_4$                        | -147                     | -136                     | -153                               | -167                                          | -63.61[ -63.63]        | -66.57                  | -66.43[ -66.36]         | -65.15                  | 0.25             |
| $3\text{C}_2\text{H}_2 \rightarrow \text{C}_6\text{H}_6$                                      | -185                     | -171                     | -215                               | -247                                          | -169.48[ -169.45]      | -172.33                 | -173.10[ -173.20]       | -154.04                 | 0.20             |
| $\text{Li}_2 + \text{F}_2 \rightarrow 2\text{FLi}$                                            | -256                     | -234                     | -251                               | -264                                          | -208.90[ -209.04]      | -215.79                 | -214.92[ -214.95]       | -216.11                 | 0.31             |
| Average $a_{\text{sys}}$                                                                      |                          |                          |                                    |                                               |                        |                         |                         |                         | 0.25             |
| MAD(kcal/mol)                                                                                 |                          |                          |                                    |                                               | 4.79[ 4.78]            | 4.51                    | 4.65[ 4.65]             |                         |                  |
| MARD(%)                                                                                       |                          |                          |                                    |                                               | 18.35[ 18.30]          | 9.62                    | 8.78[ 8.68]             |                         |                  |
| Average $a_{\text{sys}}$                                                                      |                          |                          |                                    |                                               |                        |                         |                         |                         | 0.21             |
| MAD(kcal/mol)                                                                                 |                          |                          |                                    |                                               | 5.78[ 6.18]            | 4.90                    | 4.43[ 5.08]             |                         |                  |
| MARD(%)                                                                                       |                          |                          |                                    |                                               | 57.08[ 57.79]          | 38.55                   | 35.10[ 37.49]           |                         |                  |

TABLE S.IV. Ionization potential (26 elements from the G21IP data set<sup>3</sup>) at listed reference geometries. All energies in kcal/mol. This calculation uses vdW-DF-cx orbitals for  $\Delta E^{\text{tlh}}$ , which is only meaningful for this subset of the G21IP benchmark set. Organization of data split into two subgroups depending on the nature of the vdW-DF-tlh construction, as in Table S.I.

|                               | $\Delta E_x^{\text{Fo}}$ | $\Delta E_x^{\text{cx}}$ | $\Delta E_{xc}^{\text{cx}}$ | $\Delta E_{xc,\lambda=1}^{\text{cx}}$ | $\Delta E^{\text{cx}}$ | $\Delta E^{\text{tlh}}$ | $\Delta E^{\text{cx0}}$ | $\Delta E^{\text{ref}}$ | $a_{\text{sys}}$ |
|-------------------------------|--------------------------|--------------------------|-----------------------------|---------------------------------------|------------------------|-------------------------|-------------------------|-------------------------|------------------|
| B                             | 83                       | 155                      | 174                         | 184                                   | 195[ 195]              | 186                     | 200[ 200]               | 190                     | 0.12             |
| O                             | 183                      | 189                      | 227                         | 249                                   | 317[ 317]              | 316                     | 316[ 316]               | 314                     | 0.23             |
| F                             | 226                      | 234                      | 270                         | 292                                   | 403[ 403]              | 401                     | 401[ 401]               | 402                     | 0.22             |
| Mg                            | 78                       | 80                       | 102                         | 113                                   | 173[ 173]              | 172                     | 172[ 172]               | 176                     | 0.21             |
| Al                            | 59                       | 102                      | 118                         | 125                                   | 136[ 136]              | 130                     | 140[ 140]               | 138                     | 0.13             |
| S                             | 47                       | 120                      | 154                         | 173                                   | 235[ 235]              | 224                     | 240[ 240]               | 239                     | 0.15             |
| H <sub>3</sub> N              | 160                      | 166                      | 196                         | 213                                   | 234[ 234]              | 233                     | 233[ 233]               | 236                     | 0.22             |
| HO                            | 65                       | 167                      | 201                         | 222                                   | 298[ 296]              | 284                     | 300[ 299]               | 301                     | 0.14             |
| H <sub>2</sub> O              | 198                      | 204                      | 236                         | 255                                   | 291[ 291]              | 289                     | 289[ 289]               | 293                     | 0.22             |
| HF                            | 234                      | 242                      | 275                         | 295                                   | 371[ 371]              | 369                     | 369[ 369]               | 371                     | 0.22             |
| HS                            | 78                       | 133                      | 164                         | 182                                   | 236[ 236]              | 227                     | 239[ 239]               | 239                     | 0.16             |
| C <sub>2</sub> H <sub>2</sub> | 178                      | 180                      | 210                         | 227                                   | 258[ 258]              | 258                     | 258[ 258]               | 265                     | 0.23             |
| C <sub>2</sub> H <sub>4</sub> | 175                      | 175                      | 205                         | 222                                   | 237[ 237]              | 237                     | 237[ 237]               | 244                     | 0.23             |
| Average $a_{\text{sys}}$      |                          |                          |                             |                                       |                        |                         |                         |                         | 0.19             |
| MAD(kcal/mol)                 |                          |                          |                             |                                       | 3.26[ 3.42]            | 6.62                    | 3.27[ 3.35]             |                         |                  |
| MARD(%)                       |                          |                          |                             |                                       | 1.38[ 1.44]            | 2.83                    | 1.43[ 1.45]             |                         |                  |
| H                             | 191                      | 179                      | 189                         | 193                                   | 311[ 311]              | 313                     | 314[ 314]               | 315                     | 0.24             |
| Be                            | 93                       | 87                       | 114                         | 126                                   | 206[ 206]              | 207                     | 208[ 208]               | 215                     | 0.11             |
| C                             | 226                      | 212                      | 231                         | 241                                   | 269[ 269]              | 271                     | 266[ 266]               | 260                     | 0.17             |
| Si                            | 151                      | 140                      | 155                         | 163                                   | 189[ 189]              | 190                     | 189[ 189]               | 188                     | 0.16             |
| Cl                            | 176                      | 168                      | 198                         | 216                                   | 299[ 299]              | 300                     | 299[ 299]               | 299                     | 0.15             |
| CH <sub>4</sub>               | 217                      | 197                      | 227                         | 244                                   | 286[ 286]              | 290                     | 291[ 291]               | 296                     | 0.18             |
| H <sub>4</sub> Si             | 182                      | 164                      | 194                         | 210                                   | 247[ 247]              | 250                     | 252[ 252]               | 255                     | 0.17             |
| H <sub>2</sub> P              | 165                      | 156                      | 176                         | 187                                   | 228[ 228]              | 229                     | 255[ 243]               | 226                     | 0.15             |
| H <sub>3</sub> P              | 135                      | 134                      | 162                         | 178                                   | 225[ 225]              | 225                     | 225[ 225]               | 228                     | 0.13             |
| CO                            | 187                      | 169                      | 201                         | 220                                   | 318[ 318]              | 321                     | 323[ 323]               | 323                     | 0.17             |
| N <sub>2</sub>                | 269                      | 227                      | 258                         | 276                                   | 354[ 354]              | 367                     | 365[ 365]               | 359                     | 0.30             |
| ClF                           | 202                      | 182                      | 210                         | 226                                   | 283[ 283]              | 287                     | 288[ 288]               | 292                     | 0.19             |
| CS                            | 144                      | 133                      | 163                         | 180                                   | 257[ 257]              | 259                     | 260[ 260]               | 261                     | 0.15             |
| Average $a_{\text{sys}}$      |                          |                          |                             |                                       |                        |                         |                         |                         | 0.17             |
| MAD(kcal/mol)                 |                          |                          |                             |                                       | 5.25[ 5.25]            | 4.52                    | 5.11[ 4.18]             |                         |                  |
| MARD(%)                       |                          |                          |                             |                                       | 1.95[ 1.95]            | 1.72                    | 2.07[ 1.66]             |                         |                  |
| Average $a_{\text{sys}}$      |                          |                          |                             |                                       |                        |                         |                         |                         | 0.18             |
| MAD(kcal/mol)                 |                          |                          |                             |                                       | 4.25[ 4.34]            | 5.57                    | 4.19[ 3.77]             |                         |                  |
| MARD(%)                       |                          |                          |                             |                                       | 1.66[ 1.69]            | 2.28                    | 1.75[ 1.56]             |                         |                  |

TABLE S.V. Binding energies  $\Delta E$  for molecular complexes in the S22 benchmark set,<sup>4,5</sup> at their listed reference geometries, here computed using vdW-DF-cx wavefunctions. This Table provides details behind Table III in the main text. In all of these molecular complexes, the coupling-constant scaling remains downward concave with the evaluation of  $\Delta E^{\text{tlh}}$  thus being based on Eq. (19). The results are sorted into three groups, namely, with a hydrogen bonded, dispersion bonded, or a mixed bonding character, respectively. We provide estimates of the average value for the  $\Delta E^{\text{tlh}}$  Fock-exchange mixing parameter  $a_{\text{sys}}$  for each group separately and for the entire S22 benchmark set.

|                                      | $\Delta E^{\text{Fo}}_{\text{x}}$ | $\Delta E^{\text{cx}}_{\text{x}}$ | $\Delta E^{\text{cx}}_{\text{xc}}$ | $\Delta E^{\text{cx}}_{\text{xc},\lambda=1}$ | $\Delta E^{\text{cx}}$ | $\Delta E^{\text{tlh}}$ | $\Delta E^{\text{cx0}}$ | $\Delta E^{\text{ref}}$ | $a_{\text{sys}}$ |
|--------------------------------------|-----------------------------------|-----------------------------------|------------------------------------|----------------------------------------------|------------------------|-------------------------|-------------------------|-------------------------|------------------|
| Ammonia dimer                        | 3.27                              | 2.45                              | 5.00                               | 6.84                                         | 2.63                   | 2.79                    | 2.87                    | 3.133                   | 0.20             |
| Water dimer                          | 7.18                              | 6.21                              | 8.91                               | 10.92                                        | 4.57                   | 4.77                    | 4.86                    | 4.989                   | 0.21             |
| Formic acid dimer                    | 36.28                             | 32.77                             | 42.12                              | 49.02                                        | 18.65                  | 19.38                   | 19.64                   | 18.753                  | 0.21             |
| Formamide dimer                      | 26.79                             | 23.02                             | 31.16                              | 37.07                                        | 14.93                  | 15.72                   | 15.91                   | 16.062                  | 0.21             |
| Uracil dimer h-bonded                | 26.43                             | 22.62                             | 31.98                              | 38.67                                        | 19.01                  | 19.78                   | 20.04                   | 20.641                  | 0.20             |
| 2-pyridoxine 2-aminopyridine complex | 22.07                             | 20.69                             | 30.44                              | 37.33                                        | 16.88                  | 17.13                   | 17.32                   | 16.934                  | 0.18             |
| Adenine-thymine Watson-Crick complex | 22.80                             | 20.78                             | 31.33                              | 38.73                                        | 15.45                  | 15.82                   | 16.06                   | 16.660                  | 0.18             |
| Average $a_{\text{sys}}$             |                                   |                                   |                                    |                                              |                        |                         |                         |                         | 0.20             |
| MAD(kcal/mol)                        |                                   |                                   |                                    |                                              | 0.72                   | 0.49                    | 0.43                    |                         |                  |
| MARD(%)                              |                                   |                                   |                                    |                                              | 6.78                   | 4.44                    | 3.63                    |                         |                  |
| Methane dimer                        | 1.07                              | 0.44                              | 2.12                               | 3.26                                         | 0.63                   | 0.75                    | 0.79                    | 0.527                   | 0.19             |
| Ethene dimer                         | 2.99                              | 1.23                              | 4.92                               | 7.46                                         | 0.98                   | 1.33                    | 1.42                    | 1.472                   | 0.20             |
| Benzene-methane complex              | 1.81                              | 0.42                              | 4.41                               | 7.11                                         | 1.29                   | 1.55                    | 1.65                    | 1.448                   | 0.19             |
| Benzene dimer parallel displaced     | 1.83                              | -0.65                             | 9.89                               | 16.88                                        | 2.60                   | 3.04                    | 3.25                    | 2.654                   | 0.17             |
| Pyrazine dimer                       | 3.87                              | 0.86                              | 12.08                              | 19.63                                        | 3.90                   | 4.44                    | 4.69                    | 4.255                   | 0.18             |
| Uracil dimer stack                   | 8.29                              | 2.37                              | 18.47                              | 29.32                                        | 9.30                   | 10.40                   | 10.79                   | 9.805                   | 0.19             |
| Indole-benzene complex stack         | 1.71                              | -1.81                             | 13.20                              | 23.17                                        | 4.27                   | 4.88                    | 5.18                    | 4.524                   | 0.17             |
| Adenine-thymine complex stack        | 7.86                              | 0.67                              | 23.21                              | 38.35                                        | 10.84                  | 12.15                   | 12.69                   | 11.730                  | 0.18             |
| Average $a_{\text{sys}}$             |                                   |                                   |                                    |                                              |                        |                         |                         |                         | 0.18             |
| MAD(kcal/mol)                        |                                   |                                   |                                    |                                              | 0.35                   | 0.30                    | 0.52                    |                         |                  |
| MARD(%)                              |                                   |                                   |                                    |                                              | 11.60                  | 11.98                   | 16.53                   |                         |                  |
| Ethene-ethyne complex                | 2.13                              | 1.31                              | 3.28                               | 4.62                                         | 1.54                   | 1.69                    | 1.75                    | 1.496                   | 0.19             |
| Benzene-water complex                | 4.41                              | 2.57                              | 6.72                               | 9.60                                         | 2.94                   | 3.30                    | 3.41                    | 3.275                   | 0.20             |
| Benzene-ammonia complex              | 2.86                              | 1.27                              | 5.31                               | 8.07                                         | 2.06                   | 2.36                    | 2.46                    | 2.312                   | 0.19             |
| Benzene-HCN complex                  | 6.35                              | 3.57                              | 8.68                               | 12.21                                        | 4.11                   | 4.69                    | 4.83                    | 4.541                   | 0.21             |
| Benzene dimer T-shaped               | 3.10                              | 1.00                              | 7.29                               | 11.49                                        | 2.55                   | 2.93                    | 3.09                    | 2.717                   | 0.18             |
| Indole-benzene T-shape complex       | 6.27                              | 3.26                              | 11.94                              | 17.78                                        | 5.24                   | 5.80                    | 6.01                    | 5.627                   | 0.18             |
| Phenol dimer                         | 10.13                             | 6.84                              | 15.13                              | 20.83                                        | 6.29                   | 6.92                    | 7.14                    | 7.097                   | 0.19             |
| Average $a_{\text{sys}}$             |                                   |                                   |                                    |                                              |                        |                         |                         |                         | 0.19             |
| MAD(kcal/mol)                        |                                   |                                   |                                    |                                              | 0.35                   | 0.14                    | 0.23                    |                         |                  |
| MARD(%)                              |                                   |                                   |                                    |                                              | 8.28                   | 4.71                    | 7.88                    |                         |                  |
| Average $a_{\text{sys}}$             |                                   |                                   |                                    |                                              |                        |                         |                         |                         | 0.19             |
| MAD(kcal/mol)                        |                                   |                                   |                                    |                                              | 0.47                   | 0.31                    | 0.40                    |                         |                  |
| MARD(%)                              |                                   |                                   |                                    |                                              | 9.01                   | 7.27                    | 9.68                    |                         |                  |

TABLE S.VI. Intra-molecular dissipative binding (or noncovalent intra-molecular binding) energies of the IDISP data set, at listed reference geometries.<sup>2</sup> All energies in kcal/mol, binding energies of relaxed structures are shown in brackets, where available. Reference energies from Ref. 2. The detailed reactions are<sup>2,3</sup> 1) the anthracene dimerization, 2) the 2,2-paracyclophane + 2H<sub>2</sub> to 2 p-xylene reaction, 3) the n-octane to iso-octane transformation, 4) the n-undecane to 2,2,3,3,4,4-hexamethyl-pentane transformation 5) the unfolding of C<sub>14</sub>H<sub>30</sub> and 6) the unfolding of C<sub>22</sub>H<sub>46</sub>.

|               | $\Delta E^{\text{Fo}}_{\text{x}}$ | $\Delta E^{\text{cx}}_{\text{x}}$ | $\Delta E^{\text{cx}}_{\text{xc}}$ | $\Delta E^{\text{cx}}_{\text{xc},\lambda=1}$ | $\Delta E^{\text{cx}}$ | $\Delta E^{\text{tlh}}$ | $\Delta E^{\text{cx0}}$ | $\Delta E^{\text{cx0p}}$ | $\Delta E^{\text{ref}}$ | $a_{\text{sys}}$ |
|---------------|-----------------------------------|-----------------------------------|------------------------------------|----------------------------------------------|------------------------|-------------------------|-------------------------|--------------------------|-------------------------|------------------|
| 1             | -79                               | -56                               | -109                               | -145                                         | -6.63[-6.93]           | -11.11                  | -12.50[-12.45]          | -11.31[-11.45]           | -9.15                   | 0.19             |
| 2             | -43                               | -29                               | -3                                 | 14                                           | -52.50[-52.55]         | -55.32                  | -55.67[-55.85]          | -55.05[-55.22]           | -60.28                  | 0.21             |
| 3             | 7                                 | 9                                 | -6                                 | -16                                          | -0.42[-0.42]           | -0.75                   | -0.96[-0.97]            | -0.85[-0.85]             | -1.21                   | 0.17             |
| 4             | 15                                | 17                                | -11                                | -31                                          | 10.52[10.60]           | 10.25                   | 9.95[9.99]              | 10.09[10.14]             | 9.10                    | 0.17             |
| 5             | 1                                 | 1                                 | 8                                  | 13                                           | -3.01[-2.51]           | -2.85                   | -2.74[-2.15]            | -2.80[-2.25]             | -3.64                   | 0.17             |
| 6             | 20                                | 11                                | 44                                 | 67                                           | -2.96[1.06]            | -1.32                   | -0.51[2.08]             | -1.03[1.84]              | -1.96                   | 0.18             |
| Average       |                                   |                                   |                                    |                                              |                        |                         |                         |                          |                         | 0.18             |
| MAD(kcal/Mol) |                                   |                                   |                                    |                                              | 2.36[2.73]             | 1.66                    | 1.90[2.40]              | 1.75[2.32]               |                         |                  |
| MARD(%)       |                                   |                                   |                                    |                                              | 31.52[50.64]           | 22.44                   | 28.79[53.38]            | 24.00[51.11]             |                         |                  |

TABLE S.VII. Dimerization of aluminum complexes (AL2X6) at listed reference geometries. All energies in kcal/mol. Dimerization energies at relaxed geometries are listed in brackets, where available.

|                                                                                                                | $\Delta E_x^{\text{Fo}}$ | $\Delta E_x^{\text{cx}}$ | $\Delta E_{\text{xc}}^{\text{cx}}$ | $\Delta E_{\text{xc},\lambda=1}^{\text{cx}}$ | $\Delta E^{\text{cx}}$ | $\Delta E^{\text{tlh}}$ | $\Delta E^{\text{cx0}}$ | $\Delta E^{\text{cx0p}}$ | $\Delta E^{\text{ref}}$ | $a_{\text{sys}}$ |
|----------------------------------------------------------------------------------------------------------------|--------------------------|--------------------------|------------------------------------|----------------------------------------------|------------------------|-------------------------|-------------------------|--------------------------|-------------------------|------------------|
| $\text{H}_6\text{Al}_2 \rightarrow 2\text{H}_3\text{Al}$                                                       | 26                       | 27                       | 36                                 | 43                                           | 36.6[ 36.6]            | 36.3                    | 36.4[ 36.5]             | 36.5[ 36.5]              | 38.5                    | 0.24             |
| $\text{Al}_2\text{F}_6 \rightarrow 2\text{AlF}_3$                                                              | 57                       | 42                       | 55                                 | 65                                           | 44.5[ 44.6]            | 48.7                    | 48.0[ 47.9]             | 47.3[ 47.3]              | 51.6                    | 0.29             |
| $\text{Al}_2\text{Cl}_6 \rightarrow 2\text{AlCl}_3$                                                            | 33                       | 28                       | 46                                 | 59                                           | 30.3[ 30.3]            | 31.2                    | 31.5[ 31.5]             | 31.3[ 31.3]              | 32.5                    | 0.19             |
| $\text{C}_4\text{H}_{14}\text{Al}_2 \rightarrow 2\text{C}_2\text{H}_7\text{Al}$                                | 32                       | 30                       | 43                                 | 52                                           | 36.2[ 36.2]            | 36.5                    | 36.7[ 36.7]             | 36.6[ 36.6]              | 38.4                    | 0.18             |
| $\text{C}_5\text{H}_{16}\text{Al}_2 \rightarrow \text{C}_2\text{H}_7\text{Al} + \text{C}_3\text{H}_9\text{Al}$ | 31                       | 29                       | 47                                 | 59                                           | 29.5[ 29.5]            | 29.8                    | 30.0[ 30.0]             | 29.9[ 29.9]              | 31.2                    | 0.18             |
| $\text{C}_6\text{H}_{18}\text{Al}_2 \rightarrow 2\text{C}_3\text{H}_9\text{Al}$                                | 30                       | 28                       | 50                                 | 66                                           | 22.1[ 22.0]            | 22.5                    | 22.7[ 22.7]             | 22.6[ 22.5]              | 23.1                    | 0.18             |
| Average $a_{\text{sys}}$                                                                                       |                          |                          |                                    |                                              |                        |                         |                         |                          |                         | 0.21             |
| MAD(kcal/mol)                                                                                                  |                          |                          |                                    |                                              | 2.67[ 2.67]            | 1.70                    | 1.65[ 1.67]             | 1.86[ 1.88]              |                         |                  |
| MARD(%)                                                                                                        |                          |                          |                                    |                                              | 6.81[ 6.81]            | 4.51                    | 4.21[ 4.26]             | 4.75[ 4.81]              |                         |                  |

TABLE S.VIII. Diels-Alder reaction (DARC) energies at listed reference geometries. All energies in kcal/mol. Reaction energies at relaxed geometries are listed in brackets, where available. However, the vdW-DF-cx, vdW-DF-cx0 and vdW-DF-cx0p all get the structure essentially exact and there are no discernible differences in the two sets of results.

|                                                                                                                           | $\Delta E_x^{\text{Fo}}$ | $\Delta E_x^{\text{cx}}$ | $\Delta E_{\text{xc}}^{\text{cx}}$ | $\Delta E_{\text{xc},\lambda=1}^{\text{cx}}$ | $\Delta E^{\text{cx}}$ | $\Delta E^{\text{tlh}}$ | $\Delta E^{\text{cx0}}$ | $\Delta E^{\text{cx0p}}$ | $\Delta E^{\text{ref}}$ | $a_{\text{sys}}$ |
|---------------------------------------------------------------------------------------------------------------------------|--------------------------|--------------------------|------------------------------------|----------------------------------------------|------------------------|-------------------------|-------------------------|--------------------------|-------------------------|------------------|
| $\text{C}_2\text{H}_4 + \text{C}_4\text{H}_6 \rightarrow \text{C}_6\text{H}_{10}$                                         | -102                     | -87                      | -116                               | -138                                         | -47.2[ -47.2]          | -50.5                   | -51.1[ -51.1]           | -50.3[ -50.3]            | -45.4                   | 0.22             |
| $\text{C}_2\text{H}_2 + \text{C}_4\text{H}_6 \rightarrow \text{C}_6\text{H}_8$                                            | -110                     | -97                      | -125                               | -146                                         | -65.3[ -65.3]          | -68.1                   | -68.6[ -68.6]           | -68.0[ -67.9]            | -60.8                   | 0.21             |
| $\text{C}_2\text{H}_4 + \text{C}_5\text{H}_6 \rightarrow \text{C}_7\text{H}_{10}$                                         | -83                      | -70                      | -100                               | -122                                         | -31.1[ -31.1]          | -33.8                   | -34.5[ -34.5]           | -33.8[ -33.8]            | -29.9                   | 0.21             |
| $\text{C}_2\text{H}_2 + \text{C}_5\text{H}_6 \rightarrow \text{C}_7\text{H}_8$                                            | -80                      | -72                      | -101                               | -122                                         | -37.2[ -37.2]          | -38.8                   | -39.4[ -39.3]           | -38.9[ -38.9]            | -33.6                   | 0.20             |
| $\text{C}_2\text{H}_4 + \text{C}_6\text{H}_8 \rightarrow \text{C}_8\text{H}_{12}$                                         | -89                      | -75                      | -107                               | -131                                         | -39.3[ -39.3]          | -42.2                   | -42.9[ -42.8]           | -42.1[ -42.1]            | -37.6                   | 0.20             |
| $\text{C}_2\text{H}_2 + \text{C}_6\text{H}_8 \rightarrow \text{C}_8\text{H}_{10}$                                         | -91                      | -82                      | -113                               | -136                                         | -53.7[ -53.6]          | -55.4                   | -56.0[ -56.0]           | -55.5[ -55.5]            | -49.0                   | 0.20             |
| $\text{C}_4\text{H}_4\text{O} + \text{C}_4\text{H}_2\text{O}_3 \rightarrow \text{C}_8\text{H}_6\text{O}_4(\text{endo})$   | -66                      | -49                      | -82                                | -104                                         | -12.6[ -12.7]          | -16.1                   | -17.0[ -17.0]           | -16.1[ -16.1]            | -14.0                   | 0.21             |
| $\text{C}_4\text{H}_4\text{O} + \text{C}_4\text{H}_2\text{O}_3 \rightarrow \text{C}_8\text{H}_6\text{O}_4(\text{exo})$    | -68                      | -50                      | -81                                | -104                                         | -14.2[ -14.3]          | -18.0                   | -18.8[ -18.8]           | -17.9[ -17.9]            | -15.9                   | 0.21             |
| $\text{C}_4\text{H}_4\text{O} + \text{C}_4\text{H}_3\text{NO}_2 \rightarrow \text{C}_8\text{H}_7\text{NO}_3(\text{endo})$ | -68                      | -50                      | -83                                | -106                                         | -15.4[ -15.5]          | -19.1                   | -20.0[ -20.0]           | -19.0[ -19.1]            | -16.8                   | 0.21             |
| $\text{C}_4\text{H}_4\text{O} + \text{C}_4\text{H}_3\text{NO}_2 \rightarrow \text{C}_8\text{H}_7\text{NO}_3(\text{exo})$  | -68                      | -51                      | -82                                | -105                                         | -17.3[ -17.3]          | -21.1                   | -22.0[ -22.0]           | -21.0[ -21.0]            | -18.9                   | 0.21             |
| $\text{C}_5\text{H}_6 + \text{C}_4\text{H}_2\text{O}_3 \rightarrow \text{C}_9\text{H}_8\text{O}_3(\text{endo})$           | -84                      | -66                      | -102                               | -127                                         | -31.8[ -31.9]          | -35.4                   | -36.2[ -36.2]           | -35.3[ -35.4]            | -31.7                   | 0.21             |
| $\text{C}_5\text{H}_6 + \text{C}_4\text{H}_2\text{O}_3 \rightarrow \text{C}_9\text{H}_8\text{O}_3(\text{exo})$            | -84                      | -67                      | -102                               | -127                                         | -32.3[ -32.3]          | -35.8                   | -36.6[ -36.5]           | -35.7[ -35.7]            | -32.2                   | 0.21             |
| $\text{C}_5\text{H}_6 + \text{C}_4\text{H}_3\text{NO}_2 \rightarrow \text{C}_9\text{H}_9\text{NO}_2(\text{endo})$         | -85                      | -67                      | -103                               | -128                                         | -34.3[ -34.3]          | -38.1                   | -38.8[ -38.8]           | -37.9[ -37.9]            | -34.2                   | 0.21             |
| $\text{C}_5\text{H}_6 + \text{C}_4\text{H}_3\text{NO}_2 \rightarrow \text{C}_9\text{H}_9\text{NO}_2(\text{exo})$          | -85                      | -67                      | -102                               | -127                                         | -34.6[ -34.6]          | -38.3                   | -39.0[ -39.0]           | -38.1[ -38.1]            | -34.6                   | 0.21             |
| Average $a_{\text{sys}}$                                                                                                  |                          |                          |                                    |                                              |                        |                         |                         |                          |                         | 0.21             |
| MD(kcal/mol)                                                                                                              |                          |                          |                                    |                                              | -0.84[ -0.86]          | -4.00                   | -4.74[ -4.72]           | -3.94[ -3.94]            |                         |                  |
| MAD(kcal/mol)                                                                                                             |                          |                          |                                    |                                              | 1.70[ 1.70]            | 4.00                    | 4.74[ 4.72]             | 3.94[ 3.94]              |                         |                  |
| MARD(%)                                                                                                                   |                          |                          |                                    |                                              | 5.60[ 5.52]            | 12.49                   | 15.39[ 15.35]           | 12.30[ 12.33]            |                         |                  |

TABLE S.IX. Atomization energies of the G2-1 dataset,<sup>1</sup> in kcal/mol. Atomization energies at listed reference geometries (optimized geometries) are reported outside (inside) square brackets.

|                                                  | $\Delta E^{\text{PBE0}}$ | $\Delta E^{\text{cx}}$ | $\Delta E^{\text{cx0}}$ | $\Delta E^{\text{cx0p}}$ | $\Delta E^{\text{ref}}$ |
|--------------------------------------------------|--------------------------|------------------------|-------------------------|--------------------------|-------------------------|
| LiH                                              | 52[ 52]                  | 58[ 58]                | 57[ 57]                 | 57[ 57]                  | 58                      |
| BeH                                              | 59[ 59]                  | 61[ 61]                | 62[ 62]                 | 62[ 62]                  | 50                      |
| CH                                               | 74[ 74]                  | 77[ 77]                | 71[ 72]                 | 72[ 72]                  | 84                      |
| CH <sub>2</sub> ( <sup>3</sup> B <sub>1</sub> )  | 196[ 196]                | 201[ 201]              | 196[ 196]               | 196[ 196]                | 190                     |
| CH <sub>2</sub> ( <sup>1</sup> A <sub>1</sub> )  | 185[ 196]                | 191[ 201]              | 185[ 196]               | 185[ 196]                | 181                     |
| CH <sub>3</sub>                                  | 310[ 310]                | 317[ 317]              | 311[ 311]               | 312[ 312]                | 307                     |
| CH <sub>4</sub>                                  | 418[ 418]                | 429[ 429]              | 423[ 423]               | 423[ 423]                | 420                     |
| NH                                               | 85[ 85]                  | 87[ 87]                | 84[ 84]                 | 85[ 85]                  | 84                      |
| NH <sub>2</sub>                                  | 182[ 182]                | 187[ 187]              | 182[ 182]               | 183[ 183]                | 182                     |
| NH <sub>3</sub>                                  | 293[ 293]                | 303[ 303]              | 296[ 296]               | 297[ 297]                | 298                     |
| OH                                               | 104[ 105]                | 105[ 105]              | 106[ 105]               | 107[ 107]                | 106                     |
| H <sub>2</sub> O                                 | 225[ 225]                | 237[ 237]              | 229[ 229]               | 230[ 231]                | 233                     |
| HF                                               | 136[ 137]                | 145[ 150]              | 139[ 140]               | 141[ 141]                | 141                     |
| SiH <sub>2</sub> ( <sup>1</sup> A <sub>1</sub> ) | 125[ 134]                | 155[ 155]              | 129[ 154]               | 154[ 154]                | 151                     |
| SiH <sub>2</sub> ( <sup>3</sup> B <sub>1</sub> ) | 133[ 134]                | 138[ 138]              | 137[ 138]               | 138[ 138]                | 131                     |
| SiH <sub>3</sub>                                 | 224[ 225]                | 232[ 232]              | 232[ 232]               | 232[ 232]                | 225                     |
| SiH <sub>4</sub>                                 | 315[ 316]                | 326[ 326]              | 327[ 327]               | 327[ 327]                | 322                     |
| PH <sub>2</sub>                                  | 154[ 154]                | 160[ 160]              | 158[ 158]               | 159[ 159]                | 153                     |
| PH <sub>3</sub>                                  | 238[ 238]                | 247[ 247]              | 245[ 245]               | 245[ 245]                | 242                     |
| SH <sub>2</sub>                                  | 180[ 180]                | 190[ 190]              | 183[ 183]               | 184[ 184]                | 182                     |
| HCl                                              | 104[ 104]                | 110[ 111]              | 106[ 106]               | 107[ 107]                | 106                     |
| Li <sub>2</sub>                                  | 17[ 17]                  | 19[ 19]                | 19[ 19]                 | 19[ 19]                  | 24                      |
| LiF                                              | 131[ 132]                | 140[ 145]              | 134[ 134]               | 135[ 135]                | 138                     |
| C <sub>2</sub> H <sub>2</sub>                    | 402[ 402]                | 417[ 417]              | 398[ 399]               | 400[ 401]                | 406                     |
| C <sub>2</sub> H <sub>4</sub>                    | 562[ 563]                | 579[ 579]              | 563[ 564]               | 565[ 565]                | 563                     |
| C <sub>2</sub> H <sub>6</sub>                    | 712[ 712]                | 730[ 730]              | 717[ 717]               | 718[ 718]                | 712                     |
| CN                                               | 175[ 175]                | 188[ 189]              | 168[ 168]               | 171[ 172]                | 181                     |
| HCN                                              | 305[ 307]                | 320[ 321]              | 301[ 303]               | 304[ 306]                | 313                     |
| CO                                               | 250[ 251]                | 265[ 266]              | 248[ 249]               | 250[ 252]                | 259                     |
| HCO                                              | 276[ 277]                | 294[ 294]              | 275[ 276]               | 278[ 278]                | 279                     |
| H <sub>2</sub> CO                                | 368[ 368]                | 387[ 387]              | 369[ 370]               | 372[ 372]                | 374                     |
| CH <sub>3</sub> OH                               | 506[ 507]                | 526[ 526]              | 512[ 512]               | 514[ 514]                | 513                     |
| N <sub>2</sub>                                   | 215[ 219]                | 228[ 230]              | 211[ 214]               | 214[ 217]                | 228                     |
| N <sub>2</sub> H <sub>4</sub>                    | 432[ 432]                | 449[ 450]              | 435[ 435]               | 437[ 438]                | 438                     |
| NO                                               | 147[ 147]                | 161[ 161]              | 144[ 145]               | 148[ 148]                | 153                     |
| O <sub>2</sub>                                   | 116[ 119]                | 138[ 138]              | 116[ 119]               | 121[ 123]                | 120                     |
| H <sub>2</sub> O <sub>2</sub>                    | 256[ 257]                | 281[ 281]              | 261[ 262]               | 265[ 266]                | 269                     |
| F <sub>2</sub>                                   | 31[ 32]                  | 52[ 61]                | 34[ 34]                 | 37[ 38]                  | 38                      |
| CO <sub>2</sub>                                  | 382[ 384]                | 408[ 408]              | 378[ 380]               | 383[ 385]                | 389                     |
| Na <sub>2</sub>                                  | 14[ 14]                  | 15[ 15]                | 14[ 14]                 | 14[ 14]                  | 17                      |
| Si <sub>2</sub>                                  | 76[ 77]                  | 82[ 82]                | 74[ 75]                 | 76[ 76]                  | 75                      |
| P <sub>2</sub>                                   | 110[ 111]                | 120[ 121]              | 109[ 110]               | 111[ 112]                | 117                     |
| S <sub>2</sub>                                   | 105[ 106]                | 121[ 121]              | 104[ 104]               | 106[ 106]                | 102                     |
| Cl <sub>2</sub>                                  | 58[ 58]                  | 70[ 70]                | 57[ 58]                 | 60[ 60]                  | 58                      |
| NaCl                                             | 92[ 92]                  | 96[ 96]                | 92[ 93]                 | 93[ 93]                  | 98                      |
| SiO                                              | 178[ 180]                | 195[ 195]              | 179[ 181]               | 183[ 184]                | 192                     |
| CS                                               | 165[ 165]                | 181[ 181]              | 162[ 162]               | 164[ 164]                | 171                     |
| SO                                               | 122[ 124]                | 141[ 142]              | 122[ 124]               | 125[ 126]                | 125                     |
| ClO                                              | 63[ 64]                  | 78[ 79]                | 62[ 64]                 | 66[ 67]                  | 65                      |
| ClF                                              | 58[ 59]                  | 74[ 79]                | 59[ 61]                 | 62[ 63]                  | 61                      |
| Si <sub>2</sub> H <sub>6</sub>                   | 522[ 523]                | 539[ 539]              | 538[ 539]               | 539[ 539]                | 530                     |
| CH <sub>3</sub> Cl                               | 394[ 394]                | 408[ 408]              | 396[ 397]               | 398[ 398]                | 394                     |
| CH <sub>3</sub> SH                               | 472[ 472]                | 490[ 490]              | 476[ 476]               | 478[ 478]                | 474                     |
| HOCl                                             | 158[ 159]                | 177[ 177]              | 161[ 162]               | 164[ 164]                | 164                     |
| SO <sub>2</sub>                                  | 243[ 247]                | 277[ 279]              | 243[ 247]               | 249[ 253]                | 258                     |
| MD(kcal/mol)                                     | -4.37[ -3.36]            | 8.28[ 9.09]            | -2.85[ -1.48]           | -0.61[ 0.04]             |                         |
| MAD(kcal/mol)                                    | 5.51[ 4.99]              | 8.94[ 9.73]            | 5.58[ 4.90]             | 4.18[ 4.13]              |                         |
| MARD(%)                                          | 4.42[ 4.12]              | 6.47[ 7.36]            | 4.17[ 3.68]             | 3.24[ 3.27]              |                         |

TABLE S.X. Reaction energies of the G2RC dataset<sup>2</sup> (25 reactions), in kcal/mol. Results at listed reference geometries (optimized geometries) are outside (inside) the brackets.

|                                                                                                               | $\Delta E^{\text{PBE0}}$ | $\Delta E^{\text{cx}}$ | $\Delta E^{\text{cx0}}$ | $\Delta E^{\text{cx0p}}$ | $\Delta E^{\text{ref}}$ |
|---------------------------------------------------------------------------------------------------------------|--------------------------|------------------------|-------------------------|--------------------------|-------------------------|
| $\text{C}_2\text{H}_6\text{OS} \rightarrow \text{C}_2\text{H}_4\text{S} + \text{H}_2\text{O}$                 | -2.05[ -1.55]            | 1.97[ 2.04]            | 0.07[ 0.71]             | 0.36[ 0.86]              | -2.23                   |
| $\text{CO}_2 + \text{H}_2 \rightarrow \text{CH}_2\text{O}_2$                                                  | -3.78[ -3.87]            | -0.12[ -0.13]          | -2.32[ -2.29]           | -1.87[ -1.88]            | -2.26                   |
| $\text{C}_2\text{H}_4\text{O} \rightarrow \text{CO} + \text{CH}_4$                                            | 4.03[ 4.04]              | 4.98[ 5.03]            | 3.22[ 3.23]             | 3.53[ 3.64]              | -2.18                   |
| $\text{H}_6\text{Si}_2 + \text{H}_2 \rightarrow 2\text{H}_4\text{Si}$                                         | -3.30[ -3.25]            | -1.54[ -1.50]          | -3.32[ -3.27]           | -2.97[ -2.92]            | -4.10                   |
| $\text{CO} + \text{H}_2\text{O} \rightarrow \text{CO}_2 + \text{H}_2$                                         | -13.02[ -12.95]          | -18.11[ -18.13]        | -13.46[ -13.51]         | -14.32[ -14.43]          | -7.10                   |
| $\text{C}_2\text{H}_3\text{ClO} + \text{H}_2\text{O} \rightarrow \text{C}_2\text{H}_4\text{O}_2 + \text{HCl}$ | -10.60[ -10.32]          | -8.22[ -8.18]          | -10.48[ -10.24]         | -10.04[ -9.84]           | -10.70                  |
| $\text{C}_2\text{H}_3\text{N} + \text{H}_2\text{O} \rightarrow \text{C}_2\text{H}_5\text{NO}$                 | -26.53[ -26.55]          | -27.18[ -27.16]        | -27.22[ -27.24]         | -27.15[ -27.17]          | -19.47                  |
| $\text{C}_2\text{H}_2 + \text{HF} \rightarrow \text{C}_2\text{H}_3\text{F}$                                   | -33.19[ -33.23]          | -32.98[ -33.00]        | -33.36[ -33.37]         | -33.24[ -33.35]          | -26.97                  |
| $\text{F}_2 + \text{Cl}_2 \rightarrow 2\text{ClF}$                                                            | -28.48[ -28.29]          | -27.02[ -26.71]        | -28.51[ -28.40]         | -28.18[ -28.03]          | -27.30                  |
| $\text{BCl}_3 + \text{AlF}_3 \rightarrow \text{BF}_3 + \text{AlCl}_3$                                         | -30.15[ -30.13]          | -25.51[ -25.53]        | -29.30[ -29.61]         | -28.56[ -28.58]          | -27.15                  |
| $\text{Cl}_4\text{Si} + \text{CF}_4 \rightarrow \text{F}_4\text{Si} + \text{CCl}_4$                           | -14.08[ -14.76]          | -19.11[ -19.07]        | -17.59[ -18.15]         | -17.89[ -18.35]          | -24.89                  |
| $\text{CH}_2\text{O} + \text{H}_2 \rightarrow \text{CH}_4\text{O}$                                            | -32.72[ -32.78]          | -27.25[ -27.25]        | -29.89[ -29.92]         | -29.38[ -29.40]          | -29.46                  |
| $\text{C}_2\text{H}_2 + \text{C}_2\text{H}_4 \rightarrow \text{C}_4\text{H}_6$                                | -40.66[ -40.83]          | -39.67[ -39.71]        | -40.68[ -40.79]         | -40.45[ -40.62]          | -32.71                  |
| $\text{OSi} + 3\text{H}_2 \rightarrow \text{H}_4\text{Si} + \text{H}_2\text{O}$                               | -45.10[ -44.89]          | -31.70[ -31.72]        | -39.60[ -39.32]         | -38.04[ -37.88]          | -36.32                  |
| $\text{N}_2 + 3\text{H}_2 \rightarrow 2\text{H}_3\text{N}$                                                    | -50.55[ -50.44]          | -38.79[ -38.79]        | -41.60[ -41.55]         | -41.04[ -40.87]          | -39.43                  |
| $\text{CH}_4 + 2\text{Cl}_2 \rightarrow \text{CH}_2\text{Cl}_2 + 2\text{HCl}$                                 | -46.11[ -44.73]          | -41.83[ -41.36]        | -45.74[ -44.62]         | -44.98[ -43.99]          | -48.52                  |
| $\text{C}_2\text{H}_2 + \text{H}_2 \rightarrow \text{C}_2\text{H}_4$                                          | -54.83[ -54.85]          | -50.15[ -50.16]        | -52.44[ -52.41]         | -51.98[ -52.03]          | -49.20                  |
| $\text{O}_2\text{S} + 3\text{H}_2 \rightarrow \text{H}_2\text{S} + 2\text{H}_2\text{O}$                       | -67.55[ -66.43]          | -48.19[ -48.16]        | -59.69[ -58.33]         | -57.49[ -56.50]          | -61.67                  |
| $\text{CO} + 3\text{H}_2 \rightarrow \text{H}_2\text{O} + \text{CH}_4$                                        | -75.52[ -75.51]          | -63.61[ -63.63]        | -66.43[ -66.36]         | -65.88[ -65.93]          | -65.15                  |
| $\text{F}_2\text{O} + \text{H}_2 \rightarrow \text{F}_2 + \text{H}_2\text{O}$                                 | -66.25[ -66.00]          | -56.04[ -56.01]        | -62.97[ -62.75]         | -61.70[ -61.57]          | -68.90                  |
| $\text{N}_2\text{O} + \text{H}_2 \rightarrow \text{N}_2 + \text{H}_2\text{O}$                                 | -73.69[ -73.62]          | -62.25[ -62.16]        | -73.11[ -73.04]         | -71.02[ -70.99]          | -81.21                  |
| $\text{C}_2\text{H}_4 + \text{CH}_2 \rightarrow \text{C}_3\text{H}_6$                                         | -109.84[ -98.69]         | -111.08[ -100.41]      | -109.80[ -98.65]        | -110.05[ -99.00]         | -109.11                 |
| $\text{H}_2 + \text{F}_2 \rightarrow 2\text{HF}$                                                              | -136.55[ -136.46]        | -125.82[ -125.78]      | -133.28[ -133.20]       | -131.81[ -131.72]        | -135.40                 |
| $3\text{C}_2\text{H}_2 \rightarrow \text{C}_6\text{H}_6$                                                      | -171.83[ -171.90]        | -169.48[ -169.45]      | -173.10[ -173.20]       | -172.36[ -172.65]        | -154.04                 |
| $\text{Li}_2 + \text{F}_2 \rightarrow 2\text{FLi}$                                                            | -214.79[ -214.85]        | -208.90[ -209.04]      | -214.92[ -214.95]       | -213.66[ -213.78]        | -216.11                 |
| MD(kcal/mol)                                                                                                  | -2.62[ -2.05]            | 2.16[ 2.62]            | -0.96[ -0.39]           | -0.34[ 0.19]             |                         |
| MAD(kcal/mol)                                                                                                 | 5.18[ 5.59]              | 6.16[ 6.47]            | 4.01[ 4.53]             | 4.24[ 4.72]              |                         |
| MARD(%)                                                                                                       | 29.54[ 31.00]            | 43.68[ 44.26]          | 26.43[ 28.20]           | 28.93[ 30.62]            |                         |

TABLE S.XI. Ionization potentials of the G21IP dataset<sup>3</sup> (36 elements), in kcal/mol. Results at listed reference geometries (optimized geometries) are outside (inside) the brackets.

|                               | $\Delta E^{\text{PBE0}}$ | $\Delta E^{\text{cx}}$ | $\Delta E^{\text{cx0}}$ | $\Delta E^{\text{cx0p}}$ | $\Delta E^{\text{ref}}$ |
|-------------------------------|--------------------------|------------------------|-------------------------|--------------------------|-------------------------|
| H                             | 314[ 314]                | 311[ 311]              | 314[ 314]               | 313[ 313]                | 315                     |
| Li                            | 128[ 128]                | 127[ 127]              | 128[ 128]               | 128[ 128]                | 123                     |
| Be                            | 205[ 205]                | 206[ 206]              | 208[ 208]               | 208[ 208]                | 215                     |
| B                             | 199[ 199]                | 195[ 195]              | 200[ 200]               | 200[ 200]                | 190                     |
| C                             | 266[ 266]                | 269[ 269]              | 266[ 266]               | 265[ 265]                | 260                     |
| N                             | 340[ 340]                | 343[ 343]              | 339[ 339]               | 339[ 339]                | 335                     |
| O                             | 317[ 317]                | 317[ 317]              | 316[ 316]               | 316[ 316]                | 314                     |
| F                             | 399[ 399]                | 403[ 403]              | 401[ 401]               | 402[ 402]                | 402                     |
| Na                            | 122[ 122]                | 122[ 122]              | 122[ 122]               | 122[ 122]                | 118                     |
| Mg                            | 173[ 173]                | 173[ 173]              | 172[ 172]               | 173[ 173]                | 176                     |
| Al                            | 140[ 140]                | 136[ 136]              | 140[ 140]               | 139[ 139]                | 138                     |
| Si                            | 190[ 190]                | 189[ 189]              | 189[ 189]               | 188[ 188]                | 188                     |
| P                             | 241[ 241]                | 241[ 241]              | 241[ 241]               | 241[ 241]                | 242                     |
| S                             | 240[ 240]                | 235[ 235]              | 240[ 240]               | 240[ 240]                | 239                     |
| Cl                            | 297[ 297]                | 299[ 299]              | 299[ 299]               | 298[ 298]                | 299                     |
| CH <sub>4</sub>               | 289[ 289]                | 286[ 286]              | 291[ 291]               | 290[ 290]                | 296                     |
| H <sub>3</sub> N              | 230[ 230]                | 234[ 234]              | 233[ 233]               | 233[ 233]                | 236                     |
| HO                            | 299[ 298]                | 298[ 296]              | 300[ 299]               | 301[ 299]                | 301                     |
| H <sub>2</sub> O              | 287[ 287]                | 291[ 291]              | 289[ 289]               | 289[ 289]                | 293                     |
| HF                            | 366[ 366]                | 371[ 371]              | 369[ 369]               | 369[ 369]                | 371                     |
| H <sub>4</sub> Si             | 249[ 249]                | 247[ 247]              | 252[ 252]               | 251[ 251]                | 255                     |
| HP                            | 237[ 237]                | 236[ 236]              | 236[ 236]               | 236[ 236]                | 234                     |
| H <sub>2</sub> P              | 253[ 241]                | 228[ 228]              | 255[ 243]               | 254[ 242]                | 226                     |
| H <sub>3</sub> P              | 223[ 223]                | 225[ 225]              | 225[ 225]               | 225[ 225]                | 228                     |
| HS                            | 238[ 238]                | 236[ 236]              | 239[ 239]               | 238[ 238]                | 239                     |
| HCl                           | 291[ 291]                | 293[ 293]              | 292[ 292]               | 292[ 292]                | 294                     |
| C <sub>2</sub> H <sub>2</sub> | 257[ 257]                | 258[ 258]              | 258[ 258]               | 258[ 258]                | 265                     |
| C <sub>2</sub> H <sub>4</sub> | 236[ 236]                | 237[ 237]              | 237[ 237]               | 237[ 237]                | 244                     |
| CO                            | 320[ 320]                | 318[ 318]              | 323[ 323]               | 322[ 322]                | 323                     |
| N <sub>2</sub>                | 362[ 362]                | 354[ 354]              | 365[ 365]               | 363[ 363]                | 359                     |
| O <sub>2</sub>                | 285[ 285]                | 283[ 283]              | 287[ 287]               | 286[ 286]                | 278                     |
| P <sub>2</sub>                | 239[ 238]                | 242[ 238]              | 240[ 238]               | 240[ 238]                | 243                     |
| S <sub>2</sub>                | 220[ 220]                | 216[ 216]              | 221[ 221]               | 220[ 220]                | 216                     |
| Cl <sub>2</sub>               | 259[ 259]                | 255[ 255]              | 261[ 261]               | 260[ 260]                | 265                     |
| ClF                           | 286[ 286]                | 283[ 283]              | 288[ 288]               | 287[ 287]                | 292                     |
| CS                            | 257[ 257]                | 257[ 257]              | 260[ 260]               | 259[ 259]                | 261                     |
| MD(kcal/mol)                  | -0.51[ -0.92]            | -1.66[ -1.81]          | 0.48[ 0.07]             | 0.16[ -0.25]             |                         |
| MAD(kcal/mol)                 | 4.94[ 4.68]              | 4.08[ 4.23]            | 4.13[ 3.87]             | 4.10[ 3.86]              |                         |
| MARD(%)                       | 2.09[ 1.97]              | 1.66[ 1.72]            | 1.79[ 1.67]             | 1.77[ 1.66]              |                         |

TABLE S.XII. Binding distance deviations and binding energies at energy minimum of the S22 data set. The reference binding distances are at either the CCSD(T) or MP2 level as taken from Ref. 4. The reference interaction energies are all calculated using both CCSD(T)/CBS counterpoise corrected (CP) and MP2/CBS CP as taken from Ref. 5. (Length unit: Å; energy unit: kcal/mol)

|                                      | $d^{\text{cx}} - d^{\text{ref}}$ | $d^{\text{cx0}} - d^{\text{ref}}$ | $d^{\text{cx0p}} - d^{\text{ref}}$ | $d^{\text{ref}}$ | $\Delta E^{\text{cx}}$ | $\Delta E^{\text{cx0}}$ | $\Delta E^{\text{cx0p}}$ | $\Delta E^{\text{ref}}$ |
|--------------------------------------|----------------------------------|-----------------------------------|------------------------------------|------------------|------------------------|-------------------------|--------------------------|-------------------------|
| Ammonia dimer                        | 0.100                            | 0.075                             | 0.075                              | 2.504            | 2.66                   | 2.89                    | 2.84                     | 3.133                   |
| Water dimer                          | 0.025                            | 0.025                             | 0.025                              | 1.952            | 4.57                   | 4.86                    | 4.79                     | 4.989                   |
| Formic acid dimer                    | -0.025                           | -0.025                            | -0.025                             | 1.670            | 18.68                  | 19.68                   | 19.46                    | 18.753                  |
| Formamide dimer                      | 0.000                            | -0.025                            | 0.000                              | 1.841            | 14.91                  | 15.90                   | 15.69                    | 16.062                  |
| Uracil dimer h-bonded                | -0.025                           | -0.025                            | -0.025                             | 1.775            | 18.87                  | 19.90                   | 19.68                    | 20.641                  |
| 2-pyridoxine 2-aminopyridine complex | -0.025                           | -0.025                            | -0.025                             | 1.859            | 16.91                  | 17.35                   | 17.25                    | 16.934                  |
| Adenine-thymine Watson-Crick complex | -0.025                           | -0.025                            | -0.025                             | 1.819            | 15.51                  | 16.13                   | 15.99                    | 16.660                  |
| MD                                   | 0.004                            | -0.004                            | 0.000                              |                  | -0.72                  | -0.07                   | -0.21                    |                         |
| MAD                                  | 0.032                            | 0.032                             | 0.029                              |                  | 0.72                   | 0.45                    | 0.50                     |                         |
| MARD (%)                             | 1.557                            | 1.608                             | 1.414                              |                  | 6.65                   | 3.66                    | 4.27                     |                         |
| Methane dimer                        | 0.275                            | 0.125                             | 0.125                              | 3.718            | 0.73                   | 0.82                    | 0.79                     | 0.527                   |
| Ethene dimer                         | 0.400                            | 0.275                             | 0.300                              | 3.718            | 1.34                   | 1.57                    | 1.52                     | 1.472                   |
| Benzene-methane complex              | 0.300                            | 0.150                             | 0.200                              | 2.630            | 1.45                   | 1.71                    | 1.65                     | 1.448                   |
| Benzene dimer parallel displaced     | 0.300                            | 0.200                             | 0.225                              | 3.765            | 2.98                   | 3.45                    | 3.35                     | 2.654                   |
| Pyrazine dimer                       | 0.250                            | 0.150                             | 0.175                              | 3.479            | 4.20                   | 4.85                    | 4.72                     | 4.255                   |
| Uracil dimer stack                   | 0.075                            | 0.025                             | 0.025                              | 3.365            | 9.34                   | 10.78                   | 10.49                    | 9.805                   |
| Indole-benzene complex stack         | 0.250                            | 0.150                             | 0.175                              | 3.252            | 4.63                   | 5.40                    | 5.24                     | 4.524                   |
| Adenine-thymine complex stack        | 0.100                            | 0.075                             | 0.075                              | 3.186            | 11.06                  | 12.75                   | 12.41                    | 11.730                  |
| MD                                   | 0.244                            | 0.144                             | 0.162                              |                  | -0.09                  | 0.61                    | 0.47                     |                         |
| MAD                                  | 0.244                            | 0.144                             | 0.162                              |                  | 0.24                   | 0.61                    | 0.47                     |                         |
| MARD (%)                             | 7.221                            | 4.224                             | 4.815                              |                  | 9.19                   | 20.21                   | 16.72                    |                         |
| Ethene-ethyne complex                | 0.125                            | 0.025                             | 0.025                              | 2.752            | 1.56                   | 1.76                    | 1.72                     | 1.496                   |
| Benzene-water complex                | 0.075                            | 0.000                             | 0.000                              | 2.468            | 2.95                   | 3.41                    | 3.32                     | 3.275                   |
| Benzene-ammonia complex              | 0.175                            | 0.075                             | 0.075                              | 2.583            | 2.13                   | 2.49                    | 2.42                     | 2.312                   |
| Benzene-HCN complex                  | 0.100                            | 0.025                             | 0.025                              | 2.326            | 4.14                   | 4.84                    | 4.70                     | 4.541                   |
| Benzene dimer T-shaped               | 0.175                            | 0.100                             | 0.150                              | 2.433            | 2.69                   | 3.14                    | 3.05                     | 2.717                   |
| Indole-benzene T-shape complex       | 0.150                            | 0.075                             | 0.075                              | 2.231            | 5.36                   | 6.05                    | 5.91                     | 5.627                   |
| Phenol dimer                         | 0.025                            | 0.000                             | 0.025                              | 1.937            | 6.28                   | 7.12                    | 6.94                     | 7.097                   |
| MD                                   | 0.118                            | 0.043                             | 0.054                              |                  | -0.28                  | 0.25                    | 0.14                     |                         |
| MAD                                  | 0.118                            | 0.043                             | 0.054                              |                  | 0.30                   | 0.25                    | 0.18                     |                         |
| MARD (%)                             | 4.838                            | 1.766                             | 2.244                              |                  | 6.85                   | 8.55                    | 6.20                     |                         |
| MD                                   | 0.127                            | 0.065                             | 0.076                              |                  | -0.35                  | 0.28                    | 0.15                     |                         |
| MAD                                  | 0.136                            | 0.076                             | 0.085                              |                  | 0.41                   | 0.45                    | 0.39                     |                         |
| MARD (%)                             | 4.660                            | 2.610                             | 2.915                              |                  | 7.64                   | 11.24                   | 9.41                     |                         |
